# Supplementary material for: Learning Hierarchical Relational Representations through Relational Convolutions
Source: arXiv:2310.03240 source file (2024-09-26)
Supplement: Supplementary file 1 [file appendix_efficiency.tex]

\section{Computational efficiency and parameter efficiency}\label{sec:appendix_comp_param_efficiency}
\subsection{Parameter efficiency}\label{ssec:appendix_param_efficiency}

The parameter count of both MD-IPR and relational convolution layers does not scale with the number of input objects or the number of groups considered. Instead, the parameters are shared across objects and groups. This has computational and statistical benefits. In particular, it reduces memory usage and the number of weight updates during backpropagation, as well as making the statistical estimation of a good choice of parameters easier.

\textbf{MD-IPR layer.} In a multi-dimensional inner product relation module, the parameters are the left and right projection maps, $W_1^{(k)}, W_2^{(k)} \in \reals^{d_{\mathrm{proj}} \times d_{\mathrm{in}}}, k = 1, \ldots, d_r$, where the projection dimension $d_{\mathrm{proj}}$ and the relation dimension $d_r$ are hyperparameters, and $d_{\mathrm{in}}$ is the dimensionality of the input objects (~\Cref{eq:relation_function_lin_proj}). Hence, the parameter count of a MD-IPR layer is $d_r \times d_{\mathrm{proj}} \times d_{\mathrm{in}}$. Observe that while this scales with the dimensionality of the input objects $d_{\mathrm{in}}$, it does not scale with the number of objects $m$---the same encoders are shared across all pairs of objects.

\textbf{Relational Convolution layer.} The parameters in a relational convolution layer are the graphlet filters $\bm{f} \in \reals^{s \times s \times d_r \times n_f}$. Observe that the parameter count is independent of the number of groups $\abs{\calG}$ or even the number of objects $m$. The same graphlet filters are applied to the relation subtensor corresponding to each grouping of objects. This is similar to how convolutional neural networks apply the same filters to all patches of an image. The parameter count of a relational convolution layer depends only on the filter size and number of filters, which are hyperparameters.

\subsection{Computational considerations}\label{ssec:computational_considerations}

The MD-IPR module computes an $m \times m$ relation tensor, where $m$ is the number of input objects. This quadratic computational and memory cost can be avoided under assumptions of sparsity in the discrete groups $\calG$ or group assignment matrix $G$. Such optimizations will be useful in problems involving a large number of objects.

Consider first the case relational convolution with discrete groups. The output of the relational convolution layer is $R \ast \bm{f} = \paren{\reliprod{R[g]}{\bm{f}}}_{g \in \calG}$. For each $g \in \calG$, $R[g]$ encodes the relations between objects inside of $g$. Hence, rather than computing the full $m \times m$ relation tensor, we can instead compute only,
\begin{equation*}
    \calR := \set{R_{ij} \colon \exists\, g \in \calG \text{ such that } i,j \in g}.
\end{equation*}
When $\calG$ is sparse and structured, $\calR$ is sparse.

In the case of relational convolution with (learned) soft groups, the same can be achieved via a sparse selection in the group match score $\alpha_{gk}$ (\Cref{eq:group_match_score}). The group match scores $\alpha_{gk}$ can be made sparse by using sparse normalizers like sparsemax or top-$k$ softmax, for example. Then, the relation between object $i$ and object $j$ only needs to be computed if there exists a soft group $G_k, k \in [n_g]$ which assigns non-zero weight to a discrete group $g \in \calG$ which includes both $i$ and $j$. That is,
\begin{equation*}
    \calR := \set{R_{ij} \colon \exists\, k \in [n_g], g \in \calG \text{ such that } \alpha_{gk} > 0 \text{ and } i,j \in g}.
\end{equation*}
Thus, only a sparse subset of the $m \times m$ relation tensor would need to be computed and stored.
